# Supplementary material for: The Space of Adversarial Strategies
Source: arXiv:2209.04521 source file (2023-09-06)
Supplement: Supplementary file 1 [file 10.appendix-a.tex]

\clearpage\appendix\section{Existing Attacks in Our Framework}\label{appendix-a}

\subsection{Adversarial Crafting Algorithms}\label{appendix-a:adversarial} A
core insight of this work is the generalization of attack algorithms into
constituent components that are mutually compatible with one another. To this
end, we briefly review the seminal algorithms that inspired the formulation of
our framework in \autoref{decomposition}. Throughout this overview, we will use
\(x\) to be the original sample, \(y\) as the softmax output of the network (of
\(x\)), \(\hat{y}\) to be the associated label, \(L\) to denote a loss
function, \(\alpha\) to be the perturbation magnitude, and \(x^*\) to be the
resultant adversarial example.

\shortsection{\bimfull{} (\bim{})} \bim{}~\cite{kurakin_adversarial_2016} is an
iterative extension of the \fgsmfull{}
(\fgsm{})~\cite{goodfellow_explaining_2014}. \bim{} optimizes for
\lp[\infty]-norms and perturbs samples based on the gradient of a loss function
(typically \crossentropy{}). The formulation of \bim{} is as follows:
\begin{equation*}
    x^* = x + \alpha \cdot \sign(\nabla L(y,\hat{y}))
\end{equation*}

\shortsection{\pgdfull{} (\pgd{})} \pgd{}~\cite{madry_towards_2017} is widely
regarded as the state-of-the-art attack for crafting adversarial examples.
\pgd{} is alike to \bim{} in that it also: (1) optimizes for \lp[\infty]-norms,
and (2) applies perturbations iteratively based on the gradient of the loss.
\pgd{} differentiates itself via a \textit{random restart} preprocessing step:
the optimization routine is initialized by perturbing \(x\) with a random
perturbation, drawn from a uniform distribution \(\mathcal{U}\), bounded by a
hyperparameter \(\epsilon\) (which represents the total perturbation budget).
The formulation of \pgd{} is as follows:
\begin{align*}
    x &= x + \mathcal{U}(-\epsilon, \epsilon)\\
    x^* &= x + \alpha\cdot\sign(\nabla L(y,\hat{y}))
\end{align*}

\shortsection{\jsmafull{} (\jsma{})} The
\jsma{}~\cite{papernot_limitations_2016} is unique in its definition of a
\textit{saliency map}. Built from heuristics, saliency maps encode the most
salient (\ie{} ``best'') features to perturb. Instead of using loss gradients,
the \jsma{} computes the Jacobian matrix of the model, which is then used to
build saliency maps. Finally, the \jsma{} optimizes for \lp[0]-norms, and thus,
the ``best'' single feature is selected for perturbation. The original
formulation of the saliency map used in \jsma{} (for a single feature \(i\) in
\(x\)) is as follows:
\begin{equation}
    \texttt{SM}_i\left(\dot{y},\jacobian\right) =
    \begin{dcases}
        0 & \textrm{if } J_{\dot{y},i} < 0 \textrm{ or } \sum_{j\neq\dot{y}} J_{j,i} > 0\\
        J_{\dot{y},i} \cdot \abs{\sum_{j\neq\dot{y}} J_{j,i}} & \textrm{otherwise}\\
    \end{dcases}
    \label{eq:appendix-a:jsma}
\end{equation}

\noindent where \(\jacobian{}\) is the Jacobian of the model with respect to a
sample \(x\), and \(\dot{y}\) is a target class.  Note that this saliency map
is defined for \textit{increasing} perturbations (that is, added to \(x\)); to
apply decreasing (or subtractive) perturbations, the inequalities in the
saliency map definition are inverted.

\shortsection{\dffull{} (\df{})} \df{}~\cite{moosavi-dezfooli_deepfool_2016} is
an \lp[2]-based attack which models the minimal perturbation needed to produce
adversarial examples as a projection onto the decision boundary. This
projection is defined by finding the ``closest'' class \(k\) to the label
\(\hat{y}\):
\begin{equation*}
    k = \argmin_{i \neq\hat{y}}\frac{%
        \abs{f_{\hat{y}}(x)-f_i(x)}}{\norm{\nabla f_{\hat{y}}(x)-\nabla f_i(x)}_2}
\end{equation*}

\noindent where \(f_i(x)\) is the model logit of the \(i\)th class and \(\nabla
f_i(x)\) is the \(i\)th class row of the Jacobian. The attack then perturbs
based on the logit and gradient differences of the closest class \(k\) and
label \(\hat{y}\) via:
\begin{equation}
    x^* = x + \frac{\abs{f_{\hat{y}}(x)- f_{k}(x)}}{%
        \norm{\nabla f_{\hat{y}}(x) - \nabla f_{k}(x)}_2^2}\cdot(%
            \nabla f_{\hat{y}}(x)- \nabla f_{k}(x) )
    \label{eq:appendix-a:df}
\end{equation}

\shortsection{\cwfull{} (\cw{})} Unlike other attacks which try to maximize
standard losses for model training (\eg{} \fgsm{}, \bim{}, and \pgd{}),
\cw{}~\cite{carlini_towards_2017} is unique in that it uses a custom loss function, which we
call \cwlossfull{} (\cwloss{}), to be minimized, defined as:
\begin{equation}
    \norm{\delta}_{p} + c\cdot\max(f_{\hat{y}}(x)-f_{k}(x),0)
    \label{eq:appendix-a:cwloss}
\end{equation}

\noindent where \(p\) is the target \lp{}-norm to optimize under, \(\delta\) is
defined as \(\delta=\frac{1}{2}(\tanh(w)+1)-x\) (where \(w\) is the variable
solved for), \(c\) is a hyperparameter that controls the trade-off between the
distortion introduced and misclassification, and similar to \df{}, \(k\) is the
``closest'' predicted class to the label \(\hat{y}\), as measured through the
difference of model logits between the label class \(\hat{y}\) and all other
classes.

\cw{} is unique in that it leverages a \textit{change of variables} technique
in the underlying optimization. Specifically, unlike other attacks which
optimize on \(\delta\) directly, \cw{} optimizes on \(w\), which can aid in
solving for adversarial examples~\cite{carlini_towards_2017}.

\subsection{Attack Modifications}\label{appendix-a:modifications}

\shortsection{\cwfull{}} As described in \autoref{eq:appendix-a:cwloss}, the
\cw{} attack loss function includes a hyperparameter \(c\) which controls the
trade-off between the distortion introduced and misclassification. In the
original attack definition, \(c\) is optimized dynamically through
binary-search~\cite{carlini_towards_2017}. This is cost-prohibitive and
prevents us from performing any meaningful evaluation when computational cost
is considered (as this attack would exist on a separate scale, when compared to
\pgd{} or even the \jsma{}, which requires the model Jacobian). To remedy this,
we select a constant value of \(c\) in our experiments. From the investigation
on values of \(c\) in~\cite{carlini_towards_2017} with respect to attack
success probability versus mean \lp[2] distance, we choose a value of \num{1.0}
for \(c\) in all experiments.

\shortsection{\jsmafull{}} The original definition of the \jsma{} included a
\textit{search space}, which defined the set of candidate features to be
selected for perturbation. In the original publication, the \jsma{} initially
set \(\alpha\) to either \num{1} or \num{0} (that is, pixels were fully turned
``off'' or ``on''). We find that this severely underestimates the performance
of the \jsma{} on many datasets. Instead, we derive a more effective strategy
of instead setting the saliency map score for some feature \(i\) (in an input
\(x\)) to \num{0} if: (1) the saliency score for \(i\) is positive and
\(x_i=1\), or (2) the saliency score for \(i\) is negative and \(x_i=0\). This
prevents our version of the \jsma{} from selecting features that are already at
limits of valid feature values (\ie{} \num{1} and \num{0}). Moreover, we do not
select pixel pairs, as described in~\cite{papernot_limitations_2016}, as we
found our implementation to be at least as effective (often more) as the
original \jsma{}.

\shortsection{\dlrlossfull{}} The original formulation of \dlrloss{} requires
takes the ratio of the differences between: (1) the true logit and largest
non-true-class logit, and (2) the largest logit and the third largest logit. In
our evaluation, we used datasets that had less than three classes. For those
scenarios, we take the second largest logit.
